# Supplementary material for: Range Expansion of Heterogeneous Populations
Source: arXiv:1403.6333 source file (2014-08-24)
Supplement: Supplementary file 1 [file supplement.pdf]

# Supplementary Material

In this Supplementary Material we provide additional calculations and further numerical results supporting the arguments provided in the main text.

## MAXIMUM VELOCITY IN THE DETERMINISTIC LIMIT

In this section we provide the mathematical steps to obtain the motility $\epsilon^*$ for which a homogeneous front attains the highest velocity. In the limit $\Omega \gg g(\vec{r},t) \gg 1$ the dynamics is described by partial integro-differential equations for the quantities $n_\epsilon(\vec{r},t)$ and $\rho(\vec{r},t)$

$$\partial_t n_\epsilon(\vec{r},t) = \frac{\epsilon}{2d\delta^2}\Delta n_\epsilon(\vec{r},t) + (1-\epsilon)n_\epsilon(\vec{r},t)\rho(\vec{r},t) \tag{1a}$$

$$\partial_t \rho(\vec{r},t) = -\rho(\vec{r},t)\int_0^1 (1-\epsilon)n_\epsilon(\vec{r},t)\,\mathrm{d}\epsilon\,, \tag{1b}$$

where $d \in \{1,2\}$ denotes the spatial dimension and $\Delta$ is the discrete laplacian for a lattice spacing $\delta$:

$$\Delta n_\epsilon(x,t) = n_\epsilon(x-\delta,t) + n_\epsilon(x+\delta,t) - 2n_\epsilon(x,t), \qquad d=1 \tag{2a}$$

$$\Delta n_\epsilon(r,t) = n_\epsilon(r-\delta,t) + n_\epsilon(r+\delta,t) - 2n_\epsilon(r,t) + \frac{\delta}{r}\left[n_\epsilon(r-\delta,t) - n_\epsilon(r+\delta,t)\right], \qquad d=2. \tag{2b}$$

For $d=2$ we consider a rotationally symmetric population $n_\epsilon(\vec{r},t) = n_\epsilon(r,t)$, with $r=|\vec{r}|$. According to the theory of front propagating into unstable states the front's velocity is determined by the leading edge of the front, where concentrations are low and hence $\rho(\vec{r},t)\approx 1$ [2]. At the leading edge of the front $\rho \approx 1 - \int_0^1 n_\epsilon(\vec{r},t)\,\mathrm{d}\epsilon$ holds approximately. Substituting this approximation into Eq. (1) yields

$$\partial_t n_\epsilon(\vec{r},t) \approx \frac{\epsilon}{2d\delta^2}\Delta n_\epsilon(\vec{r},t) + (1-\epsilon)n_\epsilon(\vec{r},t)\left[1 - \int_0^1 n_{\epsilon'}(\vec{r},t)\,\mathrm{d}\epsilon'\right]. \tag{3}$$

Due to the (exponential) decay of the concentrations at the leading edge, $\int_0^1 n_{\epsilon'}(\vec{r},t)\,\mathrm{d}\epsilon'$ is asympotically small and we may linearize in the concentrations:

$$\partial_t n_\epsilon(\vec{r},t) \approx \frac{\epsilon}{2d\delta^2}\Delta n_\epsilon(\vec{r},t) + (1-\epsilon)n_\epsilon(\vec{r},t). \tag{4}$$

This equation is identical to the linearized version of a Fisher equation, describing the expansion of a homogeneous population with motility $\epsilon$. We, therefore, find that at the leading edge of the front the dynamics for the different genotypes uncouples, i.e. it is described by independently propagating Fisher waves. Asymptotically, the theory of Fisher waves predicts solutions of the form $n_\epsilon(r,t) = n_\epsilon(z_\epsilon)$, with $z_\epsilon = r - v_\epsilon t$, describing a front profile propagating with velocity $v_\epsilon$ [2]. Assuming an exponentially decaying profile, $n_\epsilon(z) \sim \exp(-\gamma z) = \exp(\gamma(vt-r))$, we obtain:

$$\gamma v\, \mathrm{e}^{\gamma(\mathrm{r}-\mathrm{vt})} \approx \left[\frac{\epsilon}{2d\delta^2}\left(\mathrm{e}^{-\gamma\delta} + \mathrm{e}^{\gamma\delta} - 2\right) + (1-\epsilon)\right]\mathrm{e}^{\gamma(\mathrm{r}-\mathrm{vt})}, \qquad d=1, \tag{5a}$$

$$\gamma v\, \mathrm{e}^{\gamma(\mathrm{r}-\mathrm{vt})} \approx \left[\frac{\epsilon}{2d\delta^2}\left(\mathrm{e}^{-\gamma\delta} + \mathrm{e}^{\gamma\delta} - 2\right) + \frac{\delta}{r}\left(\mathrm{e}^{-\gamma\delta} + \mathrm{e}^{\gamma\delta}\right) + (1-\epsilon)\right]\mathrm{e}^{\gamma(\mathrm{r}-\mathrm{vt})}, \qquad d=2. \tag{5b}$$

In the limit of a large radius the terms proportional to $r^{-1}$ vanish in the Laplacian for $d=2$ and therefore both equations become identical and independent of $r$. Solving for $v$ one obtains the dispersion relation

$$v(\gamma,\epsilon) = \gamma^{-1}\left\{\frac{\epsilon}{d\delta^2}\left[\cosh(\delta\gamma) - 1\right] + 1 - \epsilon\right\}. \tag{6}$$

For fixed $\epsilon$, the solution of Eq. (3) has minimal velocity and, therefore, obeys $\frac{\partial}{\partial_\gamma}v(\gamma,\epsilon) = 0$ [1, 2]. This equation allows us to establish a relation between $\epsilon$ and $\gamma$,

$$\epsilon(\gamma) = \frac{d\delta^2}{1 + d\delta^2 - \cosh(\delta\gamma) + \delta\gamma\sinh(\delta\gamma)}. \tag{7}$$

The motility which maximizes the selected front velocity is, therefore, given by $\epsilon^* = \epsilon(\gamma^*)$, with $\gamma^*$ defined by $\frac{\mathrm{d}}{\mathrm{d}\gamma} v(\gamma, \epsilon(\gamma))\Big|_{\gamma^*} = 0$. With these results we obtain an expression for the motility maximizing the front velocity of the corresponding genotype,

$$\epsilon^* = \left[\sqrt{\frac{2}{(d\delta^2)} + 1}\ \mathrm{arccosh}\left(1 + d\delta^2\right)\right]^{-1}, \tag{8}$$

$$v^* = v(\gamma^*, \epsilon^*) = \delta \log^{-1}\left[1 + d\delta^2 + \delta\sqrt{d\left(2 + d\delta^2\right)}\right], \tag{9}$$

which is asymptotically valid in one and two spatial dimensions. For $\delta \gg 1$, one finds $\epsilon^* = (2\ln 2\delta)^{-1}$. However, in this limit a continuum approach becomes invalid since the width of the front becomes smaller than the lattice size $a$. Actually, for $\delta \gg 1$, the front speed is growth-dominated and the velocity should be equal to the growth rate times the lattice size.

## LINEAR RANGE EXPANSION IN TWO SPATIAL DIMENSIONS

In this section we investigate the planar expansion of heterogeneous populations. Specifically, we consider situations were the population is initially located on a line along the $x$-direction and the population expands towards the positive and negative $y$-direction. Figure 1 is the corresponding Figure to Fig. (1) in the main text. It shows a typical configuration of the local average motility (left) and genetic diversity (right) for a linearly expanding population.

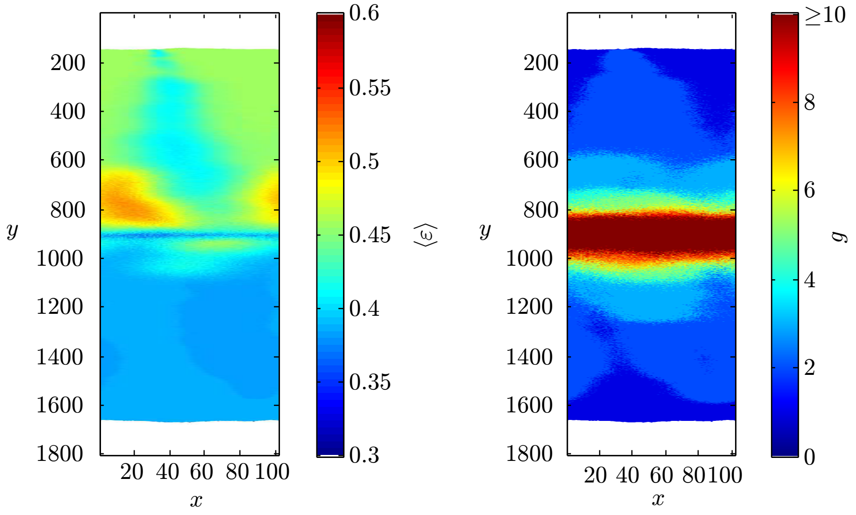


FIG. 1. Typical configuration of a linearly expanding front starting from a genetically diverse population located on the line $y = 900$ ($t = 1500$). The initial population spans the entire lattice width in $x$-direction and the 3 central lattice sites in $y$-direction. Boundary conditions are periodic in $x$-direction. Color denotes local average motility (left) and local genetic diversity (right). The downwards moving front is completely homogeneous at this time. Parameters were $\Omega = 100$ and $\delta = 1$.

Since the effect of front inflation is absent, the annihilation rate of sector boundaries is higher compared to radial fronts, leading to an early fixation of planar fronts. Consequently, the asymptotic composition of the population is biased towards a lower migration rate. In particular, due to the early fixation of the front, the average motility in the population takes a lower value than predicted by the genotype with the maximum front velocity, $\epsilon^*$. This is illustrated in Fig. 2, which shows the genetic diversity of the front $H_f$ (left) and the average motility versus time (right). Since there are two independent fronts (one in the positive and one in the negative $y$-direction), $H_f$ approaches asymptotically a value of two. In summary, the expansion of planar fronts in two spatial dimension resembles the on dimensional case in that the front fixates at an early stage of the expansion, thereby leading to the dominance of relatively slow individuals. At the same time, we observe the formation of homogeneous sectors as in the case of radially expanding populations.

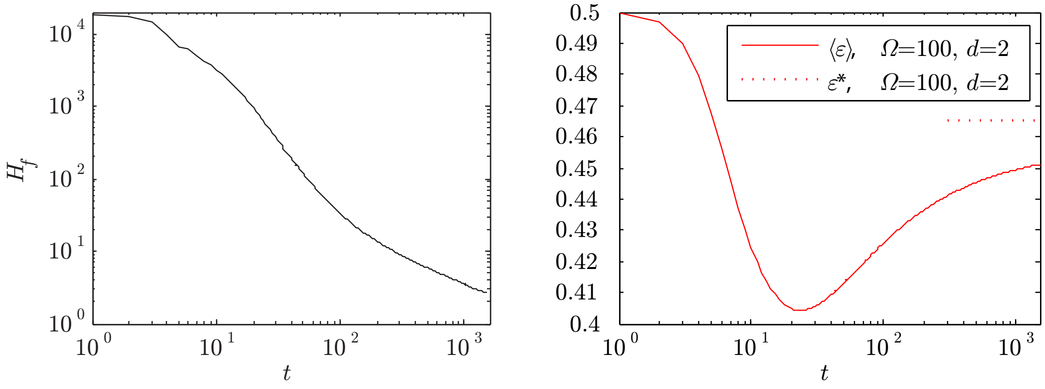


FIG. 2. Genetic diversity, $H_f$, in the front region (left) and average motility $\langle\epsilon\rangle(t)$ (right) for a planar front in two spatial dimensions (cf. the setup described in Fig. 1). The values are averaged over 400 sample runs.

## COMPARISON BETWEEN THE STOCHASTIC MODEL AND THE DETERMINISTIC LIMIT FOR $d = 1$

Figure 3 compares the evolution of the average motility in the stochastic model and the deterministic limit (given by Eqs. (1)) in one spatial dimension. The motility that asymptotically dominates the population is generally higher in one spatial dimension than in two spatial dimensions [cf. Fig. 4(a) in the main text]. Most importantly, the mean motility approaches a stationary value below the value predicted by the velocity of the fastest propagating front. The reason for this behavior is the irreversible fixation of the two front directions at an early time, where the mean motility is still relatively low.

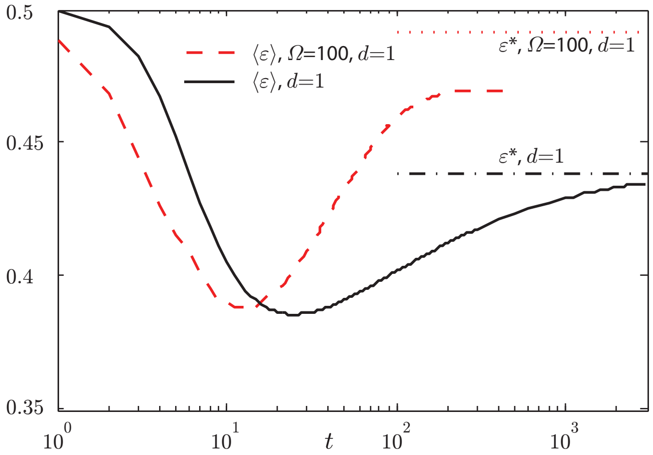


FIG. 3. Comparison of $\langle\epsilon\rangle(t)$ for simulations of the stochastic model ($\Omega = 100$) and the numerical solution of Eqs. (1), both for $\delta = 1$. The horizontal lines indicate the predicted motility $\epsilon^*$ that asymptotically dominates the population. For the stochastic model, $\epsilon^*$ is the measured value given in Fig. 4(b) in the main text.

## WIDTH OF THE FRONT

We are now interested in the width $\ell_f$ of heterogeneous fronts. To define the width of such a front we consider a point $a_f$, where the concentration of individuals drops below 0.95 and a point $b_f$, where the concentration of individuals drops below 0.05. With this, the width of the front is given by $\ell_f = b_f - a_f$.

Figure 4 shows the scaling of $\ell_f$ with the remaining free parameter, $\delta$. We find that the width of the front decreases with $\delta$ following a power law, $\ell_f \propto \delta^{-\alpha}$ with $\alpha = 0.91$, whereas for homogeneous fronts one would expect a scaling

with exponent $\alpha = 1$. In other words, the width of the front deceases more slowly as compared to the homogeneous model. The deviation from the behaviour of homogeneous fronts is most likely a consequence of the fact that for heterogeneous fronts the composition of the fronts (and thereby its shape) is itself a function of the parameter $\delta$, cf. Fig. 3 in the main text

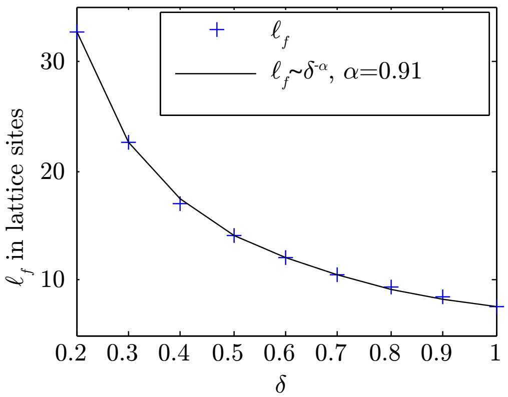


FIG. 4. Scaling of the width $\ell_f$ of a heterogeneous, stochastic front in one spatial dimension with the coarseness of the system, $\delta$. The width was measured in a time average for $180 \leq t \leq 200$ and in an ensemble average of 100 sample runs per data point for $\Omega = 1000$. The indicated fit reveals a power law decrease of the front width, $\ell_f \sim \delta^{-\alpha}$, with an exponent $\alpha = 0.91$.

## FRONT ROUGHNESS AND STOCHASTIC MOVEMENT OF SECTOR BOUNDARIES

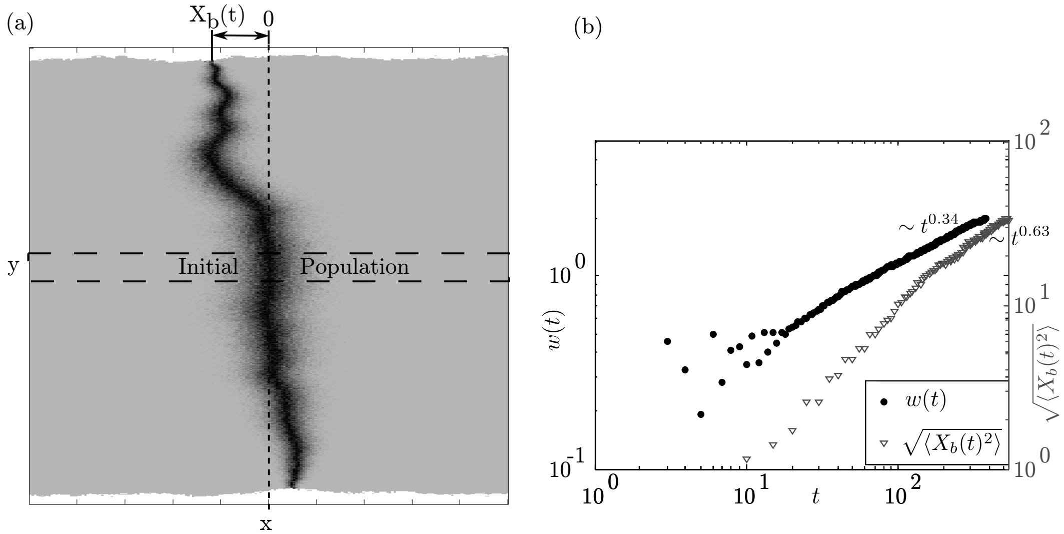


FIG. 5. (a) To study the stochastic dynamics of sector boundaries we investigated two neutral sectors of a linear front propagating in $y$-direction. Initially, the population consists of two equally sized subpopulations (dashed rectangle) with motility $\epsilon = 1/2$. Brightness represents the absolute deviation of the concentrations from 1/2, such that the sector boundary $X_b(t)$ is marked in black. Parameters of the simulation were $\delta = 1$, $\Omega = 100$, $t = 580$. (b) Root-mean-square displacement of the boundary position $X_b$ averaged over 100 simulations. Moreover the growth of the roughness $w(t)$ in a planar, homogeneous front, averaged over 500 simulations, is shown. For large times both values follow a power law. We find $\sqrt{\langle x_b^2(t) \rangle} \sim t^{\alpha}$, with $\alpha \approx 0.63$ and $w(t) \sim t^{\beta}$, with $\beta \approx 0.34$.

Does the stochastic movement of domain boundaries influence the asymptotic composition of the populations? We calculated the root-mean-square displacement of the lateral position $X_b(t)$ of a sector boundary separating two neutral genotypes, i.e. with identical mobility and reproduction rate. The computation was based on a linearly expanding

front in $d = 2$ spatial dimensions, as shown in Fig. 5(a). As there is no deterministic drift in the boundary movement we obtain $\langle X_b(t)\rangle = 0$, with the ensemble average $\langle\cdot\rangle$. Figure 5(b) shows that the root-mean-square displacement follows a power law at large times, $\sqrt{\langle x_b^2(t)\rangle} \sim t^\alpha$, with $\alpha \approx 0.63$. Since $\alpha > 0.5$ our result indicates that the meandering tangential to the front is superdiffusive. This coincides well with the observations made in Ref. [3], even though the measured growth exponent is slightly different. According to Ref. [3], this superdiffusive behavior may be attributed to the roughness of the front.

The front's roughness is defined as

$$w(t) = \sqrt{\langle [r(\varphi,t) - \langle r(\varphi,t)\rangle_\varphi]^2\rangle_\varphi} \tag{10}$$

for a radially expanding front parametrized by the polar angle $\varphi$, and as

$$w(t) = \sqrt{\langle [y(x,t) - \langle y(x,t)\rangle_x]^2\rangle_x} \tag{11}$$

for a planar front parametrized by the $x$-coordinate as shown in Fig. 5(a), respectively.

We computed the roughness for a planar, homogeneous front which ensures that the result is neither distorted by lattice artefacts nor by large scale structures from multiple sectors propagating at distinct velocities. The roughness is expected to grow according to a power law, $w(t) \sim t^\beta$ [5]. From a fit for $t \geq 100$ we obtain $\beta \approx 0.34$, confirming that homogeneous fronts as they arise in our stochastic model belong to the KPZ universality class, for which $\beta = 1/3$ [5].

[1] M. Bramson, *Convergence of solutions of the Kolmogorov equation to travelling waves* (American Mathematical Society, Providence, 1983).
[2] W. van Saarloos, Phys. Rep. **386**, 29 (2003).
[3] A. Ali and S. Grosskinsky, Adv. Complex Syst. **13**, 349 (2010).
[4] A.-L. Barabási and H. E. Stanley, *Fractal concepts in surface growth* (Cambridge university press, Cambridge, 1995).
[5] M. Kardar, G. Parisi, and Y.-C. Zhang, Phys. Rev. Lett. **56**, 889 (1986).
